# Supplementary material for: Integrated frequency-modulated optical parametric oscillator
Source: arXiv:2307.04200 source file (2023-07-09)

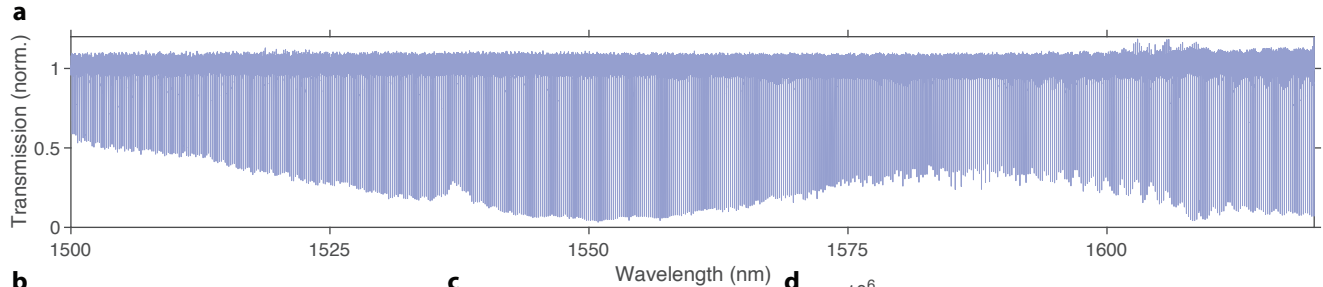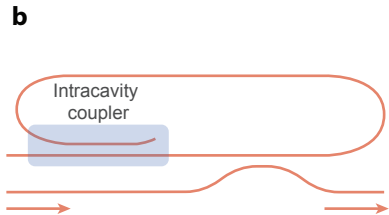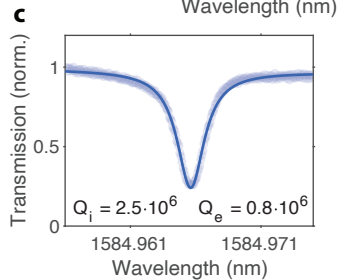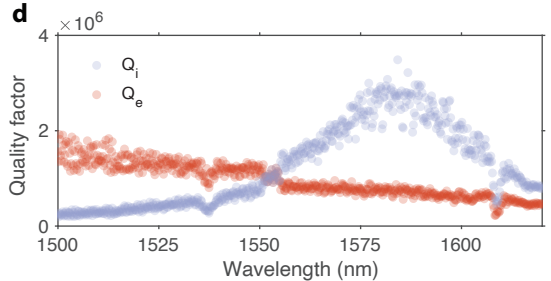

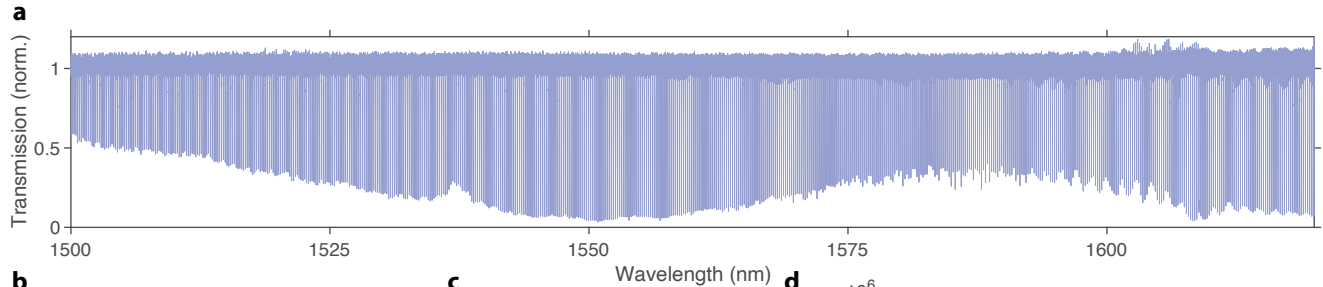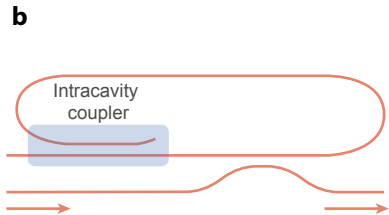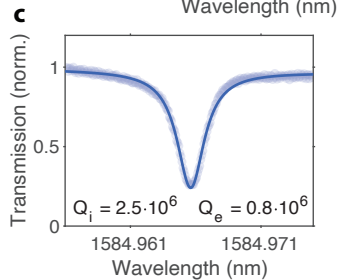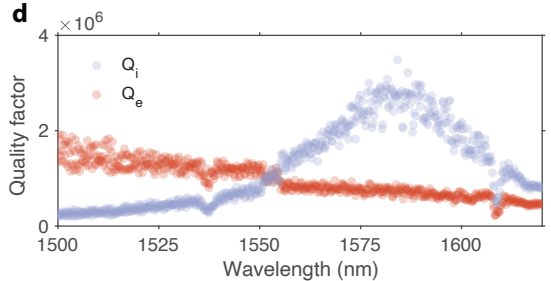

Supplement: Supplementary file 1 [file SI4.pdf]
